# Supplementary material for: A universal gate for fixed-frequency qubits via a tunable bus
Source: arXiv:1604.03076 ancillary file (2016-12-19)
Supplement: Supplementary file 1 [file swap_gate_supplement.pdf]

# Supplementary Information for "A universal gate for fixed-frequency qubits via a tunable bus"

David C. McKay,[1, a)] Stefan Filipp,[2] Antonio Mezzacapo,[1] Easwar Magesan,[1] Jerry M. Chow,[1] and Jay M. Gambetta[1]

[1)] *IBM T.J. Watson Research Center, Yorktown Heights, NY 10598, USA*

[2)] *IBM Research - Zurich, 8803 Rueschlikon, Switzerland*

(Dated: 23 November 2016)

[a)]Electronic mail: dcmckay@us.ibm.com

## I. SYSTEM SETUP

All experiments are performed at $\approx$ 10mK in a dilution refrigerator with the line configurations illustrated in Fig. 1. The qubits and high speed flux line are driven with shaped microwave pulses sequenced by an arbitrary waveform generator (TEK5014C). To generate the drive for the high speed flux line (the tunable bus drive), the signals from the generators used for the single qubit gates are mixed down to ensure phase stability and appropriate timing across experiments. The qubit state is measured in the standard way by heterodyne detection of a microwave signal reflected off CPW readout resonators coupled to each qubit. These readout resonators are at 6.8696 GHz and 6.7838 GHz respectively.

## II. SINGLE QUBIT COHERENCE AND RB

As discussed in the main text, the dressed qubits are weakly flux-tunable as given by $\tilde{\omega}_i = \omega_i + \frac{g_i^2}{\Delta_i(\Phi)}$. Flux noise on the tunable bus can therefore cause dephasing of the qubits. In Ref.[1], the relationship between $T_2^*$ and flux noise for noise power of the form $S(f) = A^2/f$, is given by the expression

$$T_2^* = \frac{1}{A}\left|\frac{\partial\omega}{\partial\phi}\right|^{-1}, \tag{1}$$

$$= \frac{1}{A}\left|\frac{g^2}{\Delta}\frac{\partial\omega_{TB}}{\partial\phi}\right|^{-1}. \tag{2}$$

To measure flux noise in our experiment we plot $T_2^*$ versus the slope of the flux tuning curve in (c) of Fig. 2. We fit the data to the function,

$$T_2^* = \frac{1}{\gamma_0 + \gamma_1 \partial\omega_{TB}/\partial\phi}, \tag{3}$$

where $\gamma_0$ accounts for decoherence from all other sources and $\gamma_1$ is the prefactor of Eqn. 2. From the fit we get that $A = 2.2 \times 10^{-4}\Phi_0$. We also measure $T_1$ and $T_2$ (echo) times for each of the qubits as a function of the DC flux. In the range measured, these quantities are not a function of flux so we infer that there is no strong Purcell effect from the coupler and that the flux noise is predominantly low frequency.

To further characterize our single qubit gates we perform randomized benchmarking (RB) of the fixed-frequency qubits with the tunable bus qubit bias at $\phi = -0.108\Phi_0$ (the flux bias for our two-qubit gate). This data is shown in (a) of Fig. 3. We perform standard RB, where

each RB experiment is run separately, and simultaneous RB, where the RB experiments and qubit measurements are performed at the same time. Simultaneous RB characterizes the level of crosstalk and spurious interaction between the qubits. As shown in (b) of Fig. 3 the spurious ZZ interaction is small at this flux bias (66kHz). Combined with the large detuning between our qubits this means that crosstalk is low and so the fidelity from simultaneous and standard RB are the same; the fidelities are 0.99909(2) and 0.99949(1) for qubits 1 and 2 respectively.

## REFERENCES

[1] J. Koch, T. M. Yu, J. Gambetta, A. A. Houck, D. I. Schuster, J. Majer, A. Blais, M. H. Devoret, S. M. Girvin, and R. J. Schoelkopf, "Charge-insensitive qubit design derived from the cooper pair box," Phys. Rev. A **76**, 042319 (2007).

**FIGURES**

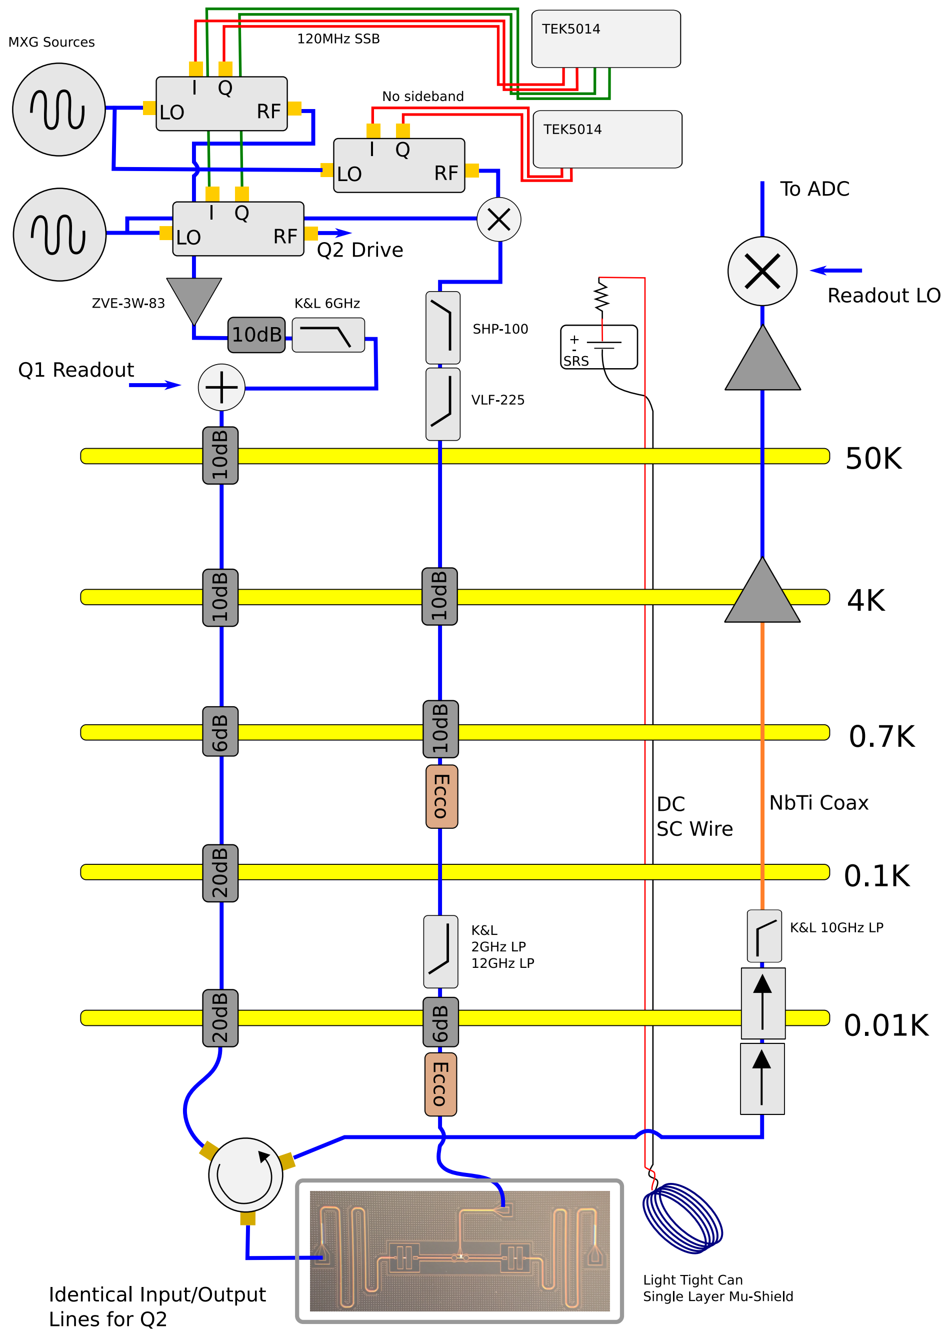


FIG. 1. Schematic of the system setup for the experiment described in the main text.

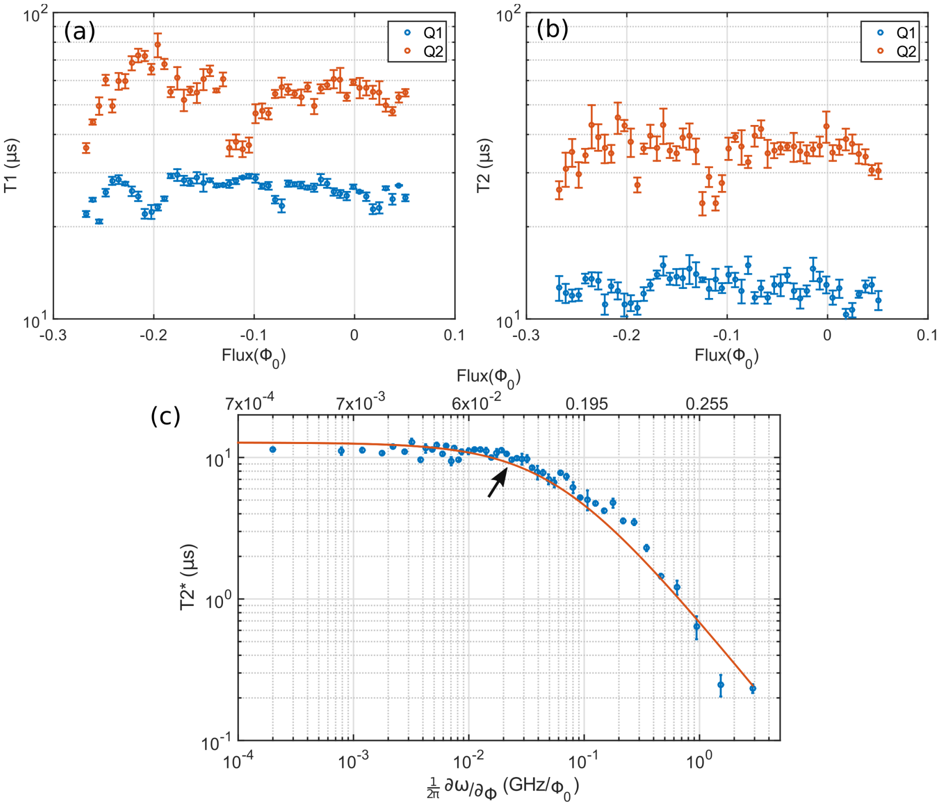


FIG. 2. Single qubit coherence measurements. (a) $T_1$ and (b) $T_2$ (echo) for both qubits as a function of the DC flux applied to the tunable bus qubit. (c) Qubit 1 $T_2^*$ as a function of the slope of the tunable bus tuning curve at specific DC flux points. The arrow indicates the point where we perform our two-qubit gate.

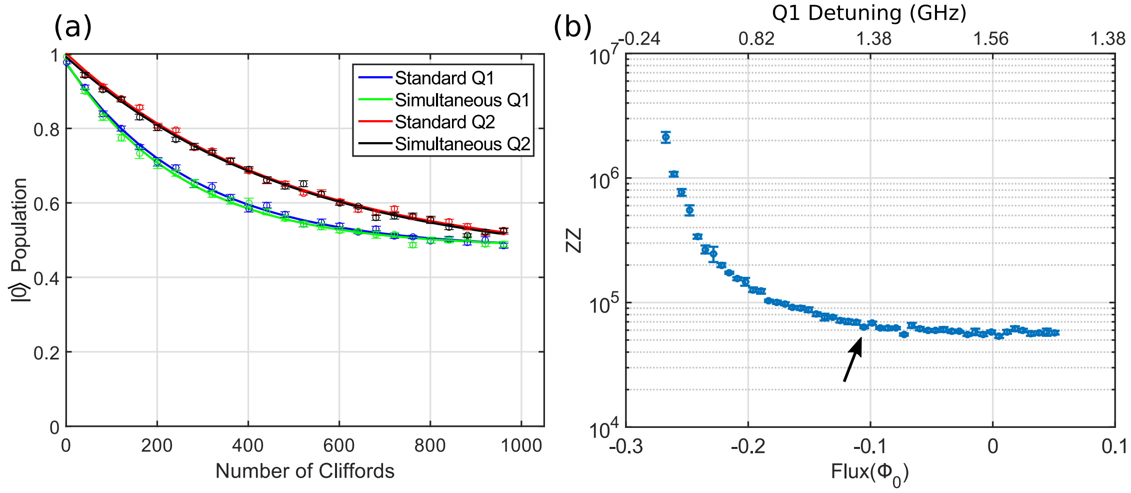


FIG. 3. (a) Standard and simultaneous RB for qubits 1 and 2 taken at the flux bias used for our two-qubit gate described in the main text. (b) ZZ Measurement as a function of DC flux bias. The arrow indicates the flux bias for our gate. For moderate detuning between qubit 1 and the tunable bus qubit (qubit 2 is always more detuned) the ZZ is low and comparable to the calculated rate of 25kHz at $\phi = 0$. The ZZ rate increases for larger flux bias as qubit 1 and the tunable bus move into resonance.
